# Supplementary material for: Leveraging active learning-enhanced machine-learned interatomic potential for efficient infrared spectra prediction
Source: arXiv:2506.13486 ancillary file (2025-06-16)
Supplement: Supplementary file 1 [file SI.pdf]

# Supplementary information for: Leveraging active learning-enhanced machine-learned interatomic potential for efficient infrared spectra prediction

Nitik Bhatia[1,2], Patrick Rinke[1,2,3,4], and Ondřej Krejčí[2,5]

[1] *Department of Physics, Technical University of Munich, James-Franck-Strasse 1, Garching, 85748, Germany*
[2] *Department of Applied Physics, Aalto University, P.O. Box 11000, AALTO, FI-00076, Finland*
[3] *Atomistic Modelling Center, Munich Data Science Institute, Technical University of Munich, Walther-Von-Dyck Str. 10, Garching, 85748, Germany*
[4] *Munich Center for Machine Learning (MCML), Munich, Germany*
[5] *Department of Mechanical and Materials Engineering, Vesilinnantie 5, Turku, Finland*

June 16, 2025

Corresponding author: patrick.rinke@tum.de

## Content

Figure S1 – A set of 24 representative small organic molecules used in this study. Figure S2 – Energy distribution of methanol, comparing DFT-based AIMD data and active learning data relative to the optimized structure. Figure S3 – Spectral similarity for 24 molecules, comparing Exp.-DFT, DFT-ML, and Exp.-ML using PCC and WD. Figure S4 – IR spectra of methanol at five temperatures, with DFT-ML similarity evaluated at each temperature using PCC and WD. Figure S5 – IR spectra of ethanol at five temperatures, with DFT-ML similarity evaluated at each temperature using PCC and WD. Figure S6 – Spectral similarity for eight organic molecules, comparing Exp.-ML spectra using PCC and WD. Figure S7 – Visualization of normal modes of methanol and sampling of structures along them. Figure S8 – Baseline correction applied to the experimental spectrum, showing improved alignment with ML predictions.

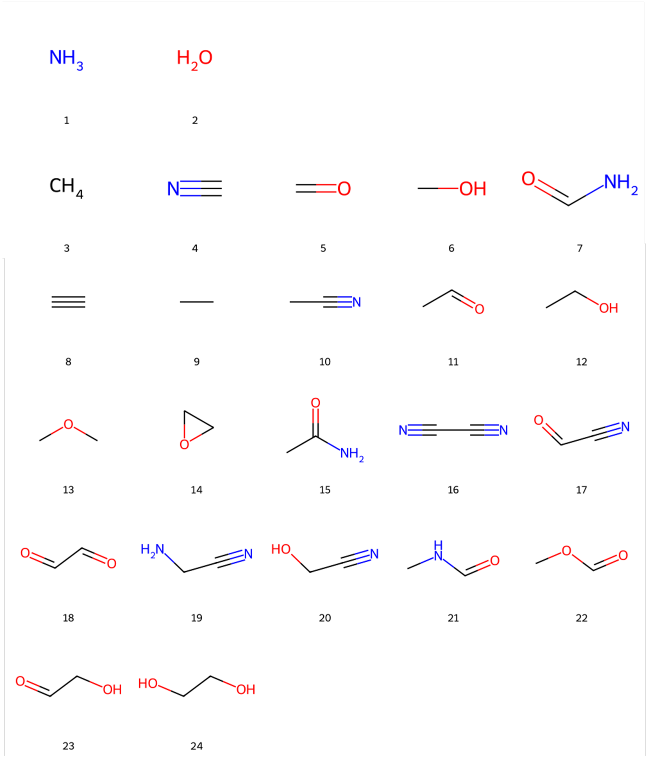


Figure S1: Visualization of the 24 small organic molecules included in this study.

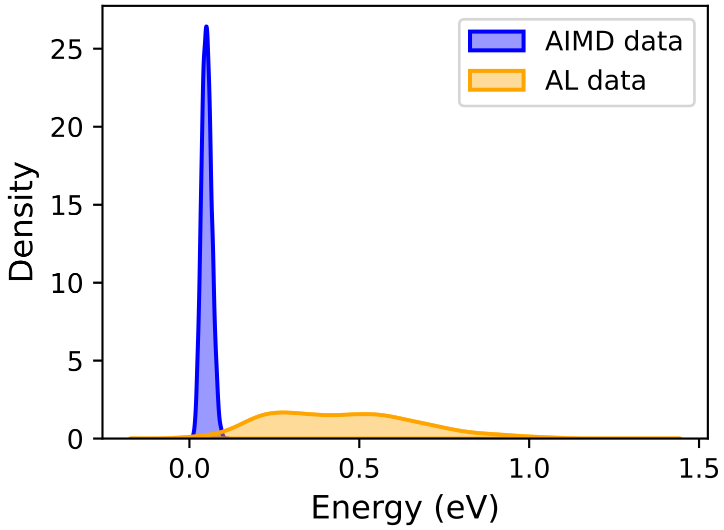


Figure S2: Energy distribution of the methanol molecule, with energies relative to the optimized structure. The data includes AIMD data (40,000 samples from DFT-based AIMD simulations) and AL data (664 samples obtained via active learning)

.

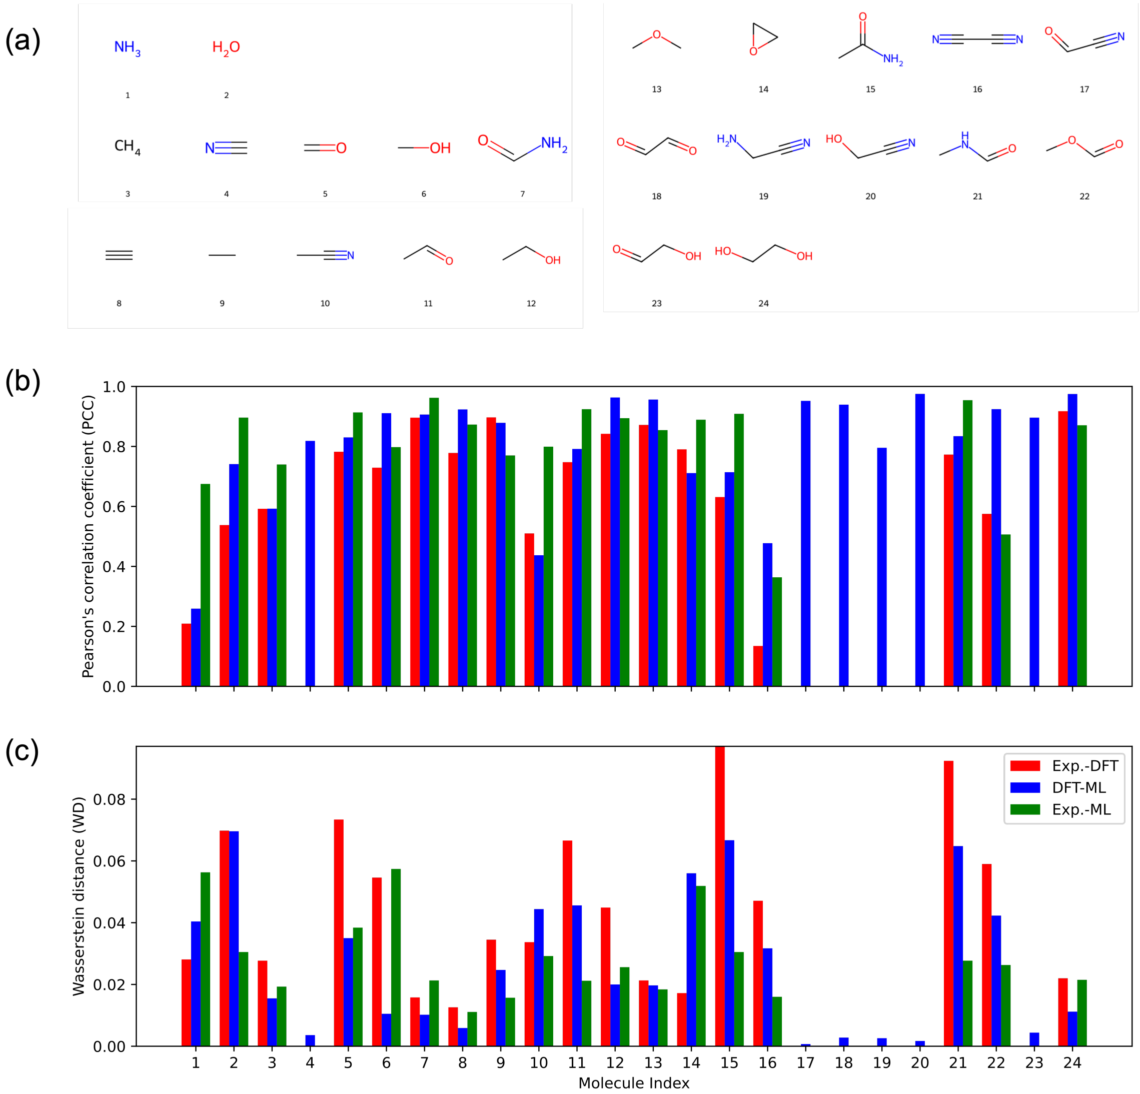


Figure S3: Spectral similarity for (a) all 24 organic molecules, comparing the pairs Exp.-DFT, DFT-ML, and Exp.-ML using (b) Pearson's correlation coefficient (PCC) and (c) Wasserstein distance (WD). For six molecules (indices 4, 17, 18, 19, 20, and 23), experimental spectra are unavailable, so only the DFT-ML comparison is provided for these cases.

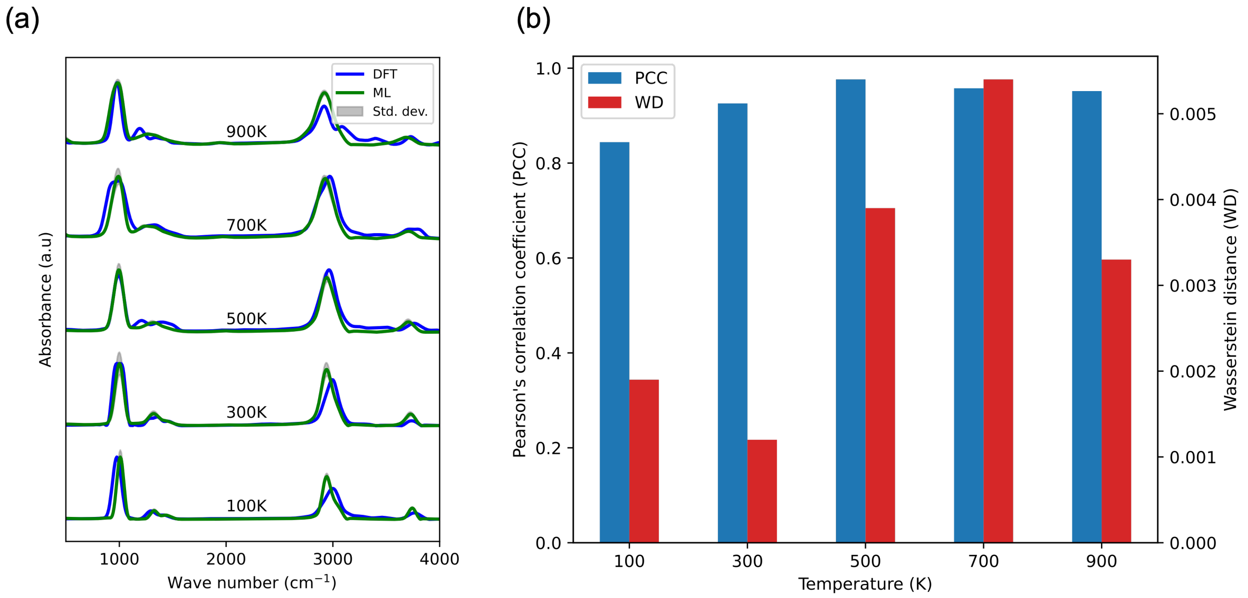


Figure S4: (a) IR spectra of methanol at five different temperatures: 100K, 300K, 500K, 700K, and 900K. (b) Spectral similarity at each temperature between DFT-ML predictions, evaluated using Pearson's correlation coefficient (PCC) and Wasserstein distance (WD).

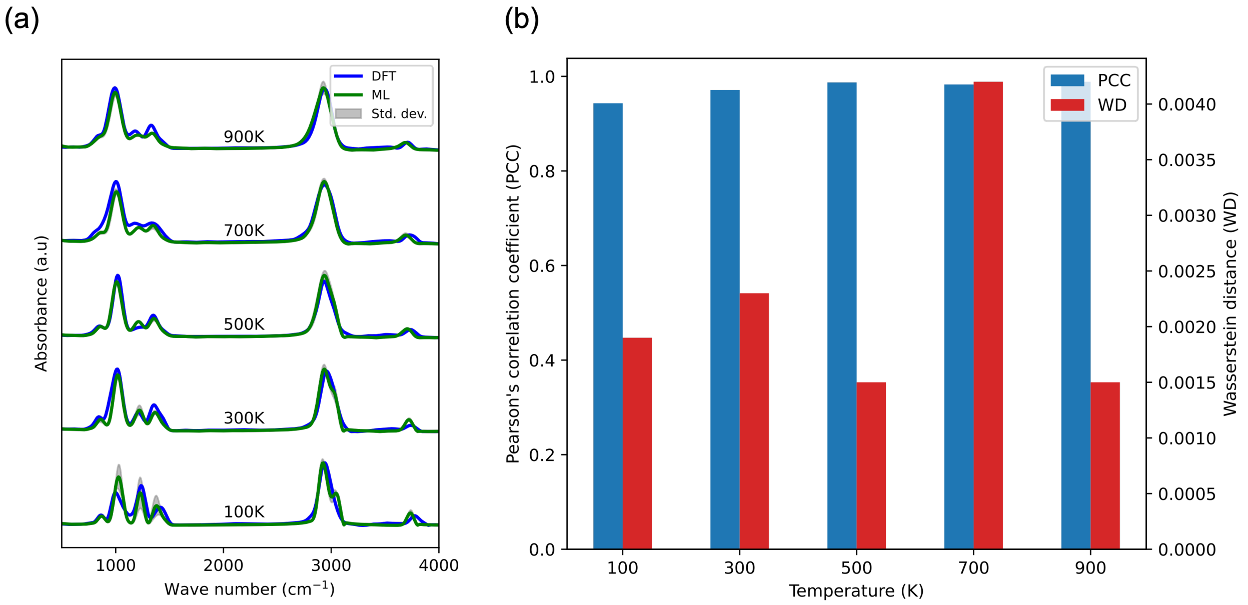


Figure S5: (a) IR spectra of ethanol at five different temperatures: 100K, 300K, 500K, 700K, and 900K. (b) Spectral similarity at each temperature between DFT-ML predictions, evaluated using Pearson's correlation coefficient (PCC) and Wasserstein distance (WD).

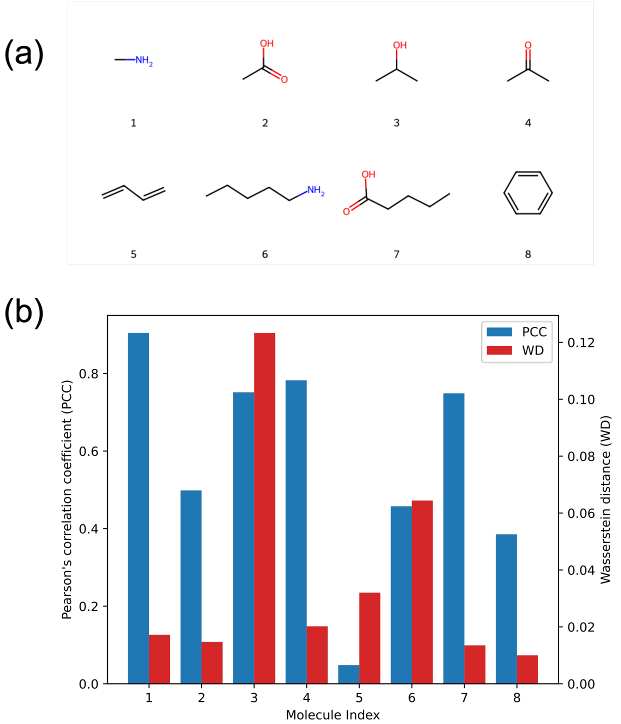


Figure S6: Spectral similarity for (a) eight organic molecules, distinct from the training data or featuring increasing carbon atoms and varying functional groups, (b) evaluated between Exp.-ML predictions using Pearson's correlation coefficient (PCC) and Wasserstein distance (WD).

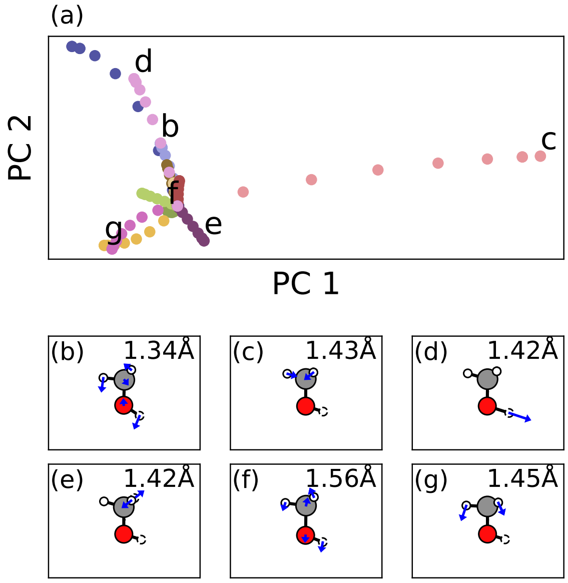


Figure S7: (a) Principal component analysis (PCA) on global Smooth Overlap of Atomic Positions [1,2] (SOAP) features of methanol structures. The filled circles in the same color are the structures along one specific mode and different color indicates different modes. (b)-(g) Snapshots of the selected structures. The normal vectors are plotted in blue arrows and C-O bond length is labeled [3].

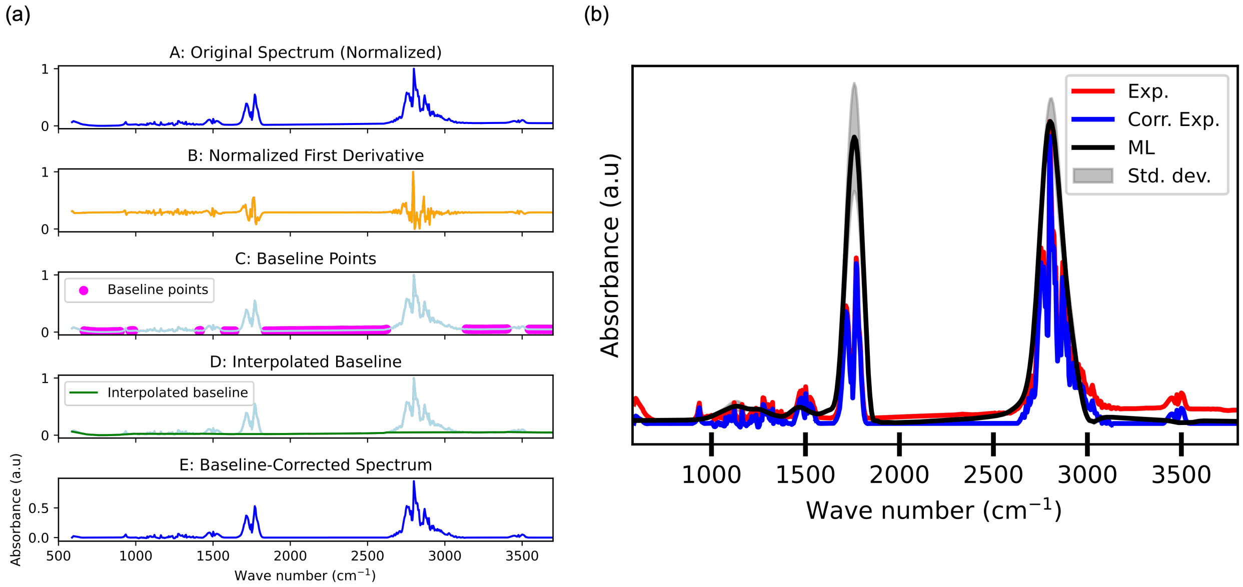


Figure S8: (a) Baseline correction procedure [4] for the IR spectrum of formaldehyde. The method involves several steps, starting from (A) Original IR spectrum of formaldehyde. (B) First derivative of the spectrum. Data points where derivative is exceeding a threshold (0.0008) and their neighboring points are identified and excluded from baseline points labeling. (C) Remaining data points used for baseline fitting are marked in magenta. (D) Linear interpolation (green line) is used to create the baseline. (E) Final baseline-corrected spectrum after subtraction of the baseline.
(b) Comparison of the original experimental IR spectrum, the baseline-corrected spectrum, and the ML-predicted spectrum for formaldehyde. The baseline correction removes distortions, enhancing the alignment between the experimental and ML spectra.

# References

[1] Sandip De, Albert P. Bartók, Gábor Csányi, and Michele Ceriotti. Comparing molecules and solids across structural and alchemical space. *Phys. Chem. Chem. Phys.*, 18:13754–13769, 2016.

[2] Lauri Himanen, Marc O.J. Jäger, Eiaki V. Morooka, Filippo Federici Canova, Yashasvi S. Ranawat, David Z. Gao, Patrick Rinke, and Adam S. Foster. Dscribe: Library of descriptors for machine learning in materials science. *Computer Physics Communications*, 247:106949, 2020.

[3] Zeyuan Tang, Stefan T. Bromley, and Bjørk Hammer. A machine learning potential for simulating infrared spectra of nanosilicate clusters. *The Journal of Chemical Physics*, 158(22):224108, June 2023.

[4] Beatriz von der Esch, Laurens D. M. Peters, Lena Sauerland, and Christian Ochsenfeld. Quantitative Comparison of Experimental and Computed IR-Spectra Extracted from Ab Initio Molecular Dynamics. *Journal of Chemical Theory and Computation*, 17(2):985–995, 2021.
